# Supplementary material for: Stability of even-denominator fractional quantum Hall states in systems with strong Landau-level mixing
Source: arXiv:2109.14773 source file (2021-09-30)
Supplement: Supplementary file 1 [file supplementary.pdf]

# Stability of even-denominator fractional quantum Hall states in strong Landau-level-mixed systems — supplementary materials

Wenchen Luo,[1] Shenglin Peng,[2,1] Hao Wang,[3] Yu Zhou,[4] and Tapash Chakraborty[5,6]

[1]*School of Physics and Electronics, Central South University, Changsha, China 410083*
[2]*School of Information Science and Technology, Northwest University, Xi'an, China 710127*
[3]*Shenzhen Institute for Quantum Science and Engineering, Southern University of Science and Technology, Shenzhen, China 518055*
[4]*Department of Physics, Jiangsu University of Science and Technology, Jiangsu, China 212003*
[5]*Department of Physics, Brock University, St. Catharines, ON, Canada L2S 3A1*
[6]*Department of Physics and Astronomy, University of Manitoba, Winnipeg, Canada R3T 2N2*
(Dated: August 14, 2021)

### A. Density response function of the 2DEG in an infinite square well

If we consider higher bands $m_i > 1$ but without inter-band interaction, then the Coulomb interaction matrix element is

$$V_{(s),i_1,i_2,i_3,i_4}^{m;n_1,n_2,n_3,n_4} = \frac{e^2}{\epsilon\ell}\frac{2}{\pi N_s}\overline{\sum_{\mathbf{q}}} V_{i_1,i_2,i_3,i_4}^{n_1,n_2,n_3,n_4}(\mathbf{q})\int_0^\infty \frac{dq_z\ell}{\epsilon_s(q,q_z)(q^2+q_z^2)\ell^2}\frac{32\pi^4\left[1-\cos(q_zL_z/m)\right]}{\left(4\pi^2 q_zL_z/m - q_z^3L_z^3/m^3\right)^2}, \tag{S1}$$

where $m = m_i$ is the band index.

The noninteracting retarded density-density response function computed in random phase approximation $\chi_{nn}^0(q,q_z,\omega)$ is related to the bare bubble in the Feynman diagram. If we do not consider the disorders in a high quality sample, then the response function can be simplified in the static limit,

$$\begin{aligned}\chi_{nn}^0(q,q_z) &\equiv \chi_{nn}^0(q,q_z,\omega\to 0)\\ &= \frac{1}{2\pi\ell^2L_z}\sum_\sigma\sum_{m_1,n_1}\sum_{m_2,n_2}\left|G_{m_2,n_2}^{m_1,n_1}(q,q_z)\right|^2\frac{\nu_{(m_1,n_1),\sigma}-\nu_{(m_2,n_2),\sigma}}{E_{(m_1,n_1),\sigma}-E_{(m_2,n_2),\sigma}},\end{aligned} \tag{S2}$$

where $E_{(m_1,n_1),\sigma}$ and $\nu_{(m_1,n_1),\sigma}$ are the kinetic energy and filling factor of LL $(m_1,n_1)$ with spin $\sigma$, respectively. The response function is similar to the two-dimensional case, while the $z$ component of the system needs to be integrated in the form factor. The from factor is

$$G_{m_2,n_2}^{m_1,n_1}(q,q_z) = F_{n_1,n_2}(-\mathbf{q})\frac{iq_zL_z}{\pi^2}g_{m_1,m_2}(-q_z) \tag{S3}$$

with the functions

$$F_{n,n'}(\mathbf{q}) = \frac{\sqrt{\min(n,n')!}}{\sqrt{\max(n,n')!}}e^{-\frac{q^2\ell^2}{4}}L_{\min(n,n')}^{|n-n'|}\left(\frac{q^2\ell^2}{2}\right)\left[\frac{\mathrm{sgn}(n-n')q_y\ell+iq_x\ell}{\sqrt{2}}\right]^{|n-n'|} \tag{S4}$$

$$g_{m_1,m_2}(q_z) = \left[1-e^{iq_zL}\cos(m_1-m_2)\pi\right]\left[\frac{1}{(m_1-m_2)^2-\frac{q_z^2L_z^2}{\pi^2}}-\frac{1}{(m_1+m_2)^2-\frac{q_z^2L_z^2}{\pi^2}}\right], \tag{S5}$$

where $L$ is a Laguerre polynomial.

If more than one LLs are considered in the Hamiltonian, then the correlations between these LLs in the response function should be omitted to avoid the double counting. Suppose that the considered $k$ LLs in the Hamiltonian are in the set $M = \{(M_1,N_1),(M_2,N_2),\ldots(M_k,N_k)\}$, then $(m_1,n_1)$ and $(m_2,n_2)$ in the summation in Eq. (S2) can not belong to the set $M$ at the same time.

### B. Coulomb interaction matrix element in a conventional 2DEG

In a conventional quantum well, such as GaAs, if the width of the well is supposed to be zero, and the electron gas is supposed to be exact two-dimensional. In the rectangle geometry with the periodic boundary condition, the Coulomb interaction matrix element is given by

$$V_{i_1,i_2,i_3,i_4}^{n_1,n_2,n_3,n_4}(\mathbf{q}) = \delta'_{i_1,i_4+q_y\ell^2}\delta'_{i_2,i_3-q_y\ell^2}e^{iq_x(i_3-i_1)}F_{n_1,n_4}(\mathbf{q})F_{n_2,n_3}(-\mathbf{q}), \tag{S6}$$

where the function $F$ is given by Eq. (S4) and $\delta'$ includes the periodic boundary condition,

$$\delta'_{i_1,i_2} = \begin{cases} 1, & \mathrm{mod}\,(i_1 - i_2, N_s) = 0 \\ 0, & \mathrm{mod}\,(i_1 - i_2, N_s) \neq 0 \end{cases} .$$

### C. Screening Coulomb potential matrix in a multi-layer system

The wave function of a bilayer 2DEG can be generally written as $\psi_n^{BL}(\mathbf{r}) = \begin{pmatrix} \psi_n^1(\mathbf{r}) & \psi_n^2(\mathbf{r}) \end{pmatrix}^{\mathrm{T}}$ where the two components of the spinor represent the wave functions in two different layers. The unscreened Coulomb potential should be written in a matrix form,

$$V(q) = \frac{1}{q\ell} \begin{pmatrix} 1 & e^{-qd} \\ e^{-qd} & 1 \end{pmatrix}, \tag{S7}$$

where $d$ is the distance between the two layers. The bubble diagram is defined by the density response function, in which the form factor is $G_{n_2}^{n_1}(\mathbf{q}) = \Phi^1_{n_1,n_2}(\mathbf{q}) + \Phi^2_{n_1,n_2}(\mathbf{q})$ with the Fourier transform of the density factor of layer $i$, $\Phi^i_{n_1,n_2}(\mathbf{q}) = \int d\mathbf{r}\, \psi^{i*}_{n_1}(\mathbf{r})\, \psi^i_{n_2}(\mathbf{r})\, e^{-i\mathbf{q}\cdot\mathbf{r}}$. The bare bubble is then divided into four parts $(i,j = 1,2)$,

$$\Pi_{ij}(\mathbf{q}) = \frac{e^2}{\epsilon\ell} \sum_{\sigma,n_1,n_2} \Phi^{i*}_{n_1,n_2}(\mathbf{q})\, \Phi^{j}_{n_1,n_2}(\mathbf{q})\, \frac{\nu_{n_1,\sigma} - \nu_{n_2,\sigma}}{E_{n_2,\sigma} - E_{n_1,\sigma}}, \tag{S8}$$

and the screened Coulomb potential reads

$$V^s(q) = \frac{\frac{1}{q\ell}\begin{pmatrix} 1 & e^{-qd} \\ e^{-qd} & 1 \end{pmatrix}}{1 + \begin{pmatrix} \Pi_{11} & \Pi_{12} \\ \Pi_{21} & \Pi_{22} \end{pmatrix} \frac{1}{q\ell} \begin{pmatrix} 1 & e^{-qd} \\ e^{-qd} & 1 \end{pmatrix}}, \tag{S9}$$

where $d$ is the distance between the two layers. We note that the screened intra-layer Coulomb potentials are not necessarily the same, since the densities in different layers may be different, while the inter-layer potentials are always similar $(V^s_{12} = V^s_{21})$.

This formula can be generalized to multi-layer systems, the Coulomb potential matrix has dimensions the same as the number of layers.

For black phosphorene, the single-particle wave function is given in Eq. (4) in the main text, so the Coulomb potentials $V^s_{11}, V^s_{12}$ can be obtained by inserting the form factors $\Phi^{1,2}_{n_1,n_2}(\mathbf{q}) = \frac{1}{2}\sum_{m',m}\left(u^*_{n_1,m'}u_{n_2,m} + v^*_{n_1,m'}v_{n_2,m}\right) F_{m',m}(-\mathbf{q})$ into Eq. (S9).

### D. More numerical data in ZnO quantum well

Besides the numerical results shown in the main text, we supplement some data for the ZnO quantum well.

Fig. S1 shows the same phase diagram as that in Fig. 1. The difference is that there are only 7 electrons here.

Fig. S2 shows the same phase diagram as that in Fig. 2. The difference is that there are only 7 electrons here. It is clear that the phase diagrams are not changed too much by the effective mass. The gaps are slightly decreased by increasing electron number.

To convince that the incompressibility can be survived in sample a, we perform the exact diagonalization in a larger system. We select LLs $N = 0, 1, 2$ in the many-body Hamiltonian, and the total electron number $N_e = 15$ with $N_s = 10$ in a single LL. We can find that the 2DEG is incompressible when half-width of the wave function $W > 5.4$ nm. Fig. S3 shows the collective modes in such a system.

Moreover, the arc region where the 2DEG is incompressible looks like to be bonded by a quantity $B \cdot W$, where $W$ is the half width of the wave function. We may judge a system incompressible or not by this quantity. Based on the gap data shown in Fig. 2 in the main text, we have the following Fig. S4 showing the relation between $B \cdot W$ and the minimum gap. It is clear that when $B \cdot W < 30$ T·nm, the 2DEG is likely compressible.

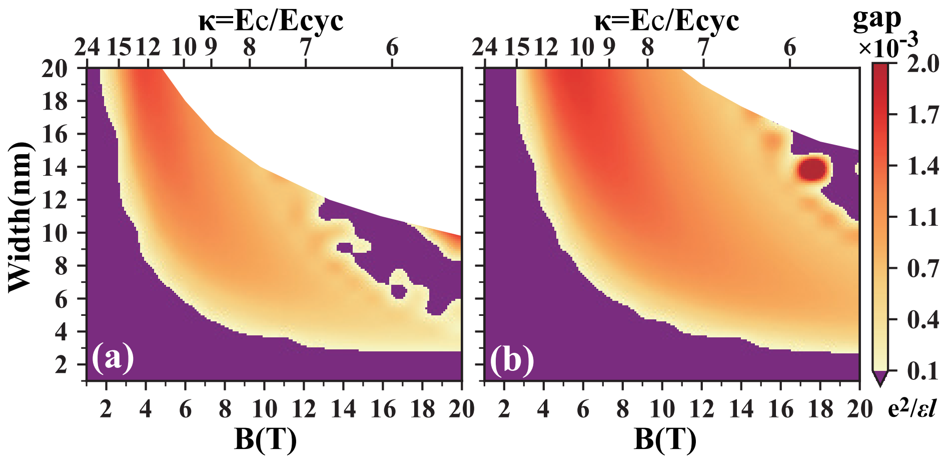


FIG. S1: The lowest gaps in the collective modes (phase diagram) in different magnetic fields and widths of the ZnO quantum well. $m^* = 0.44m_e$ and $\epsilon = 8.5$. The confinements of the 2DEG in the $z$ direction are (a) parabolic potential and (b) infinite square well. Electron number $N_e = 7$.

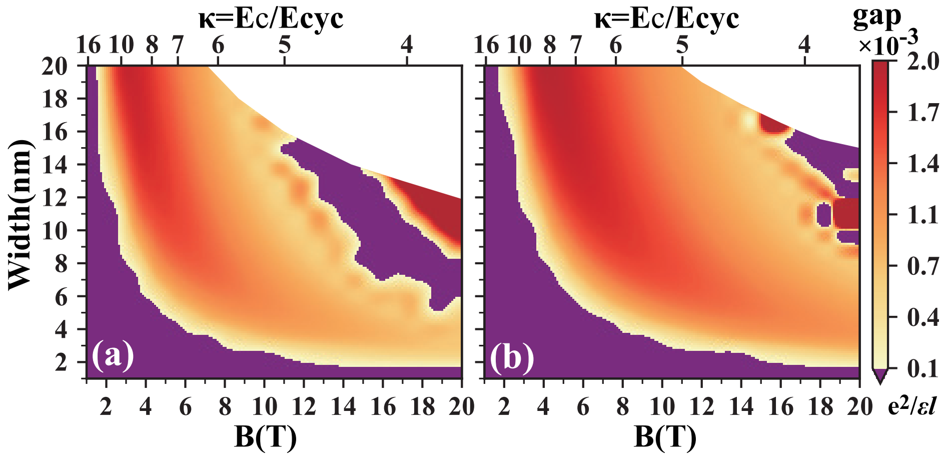


FIG. S2: The lowest gaps in the collective modes (phase diagram) in different magnetic fields and widths of the ZnO quantum well. $m^* = 0.3m_e$ and $\epsilon = 8.5$. The confinements of the 2DEG in the $z$ direction are (a) parabolic potential and (b) infinite square well. Electron number $N_e = 7$.

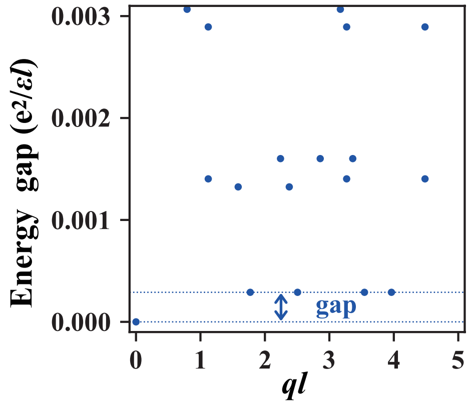


FIG. S3: The collective modes with parameters of sample a in Ref.[1] which are also given in the main text. A gap is shown to stabilize the incompressibility. Width of the wave function is $W = 17/3$ nm and the width of quantum well is $L_z = 8.5$ nm.

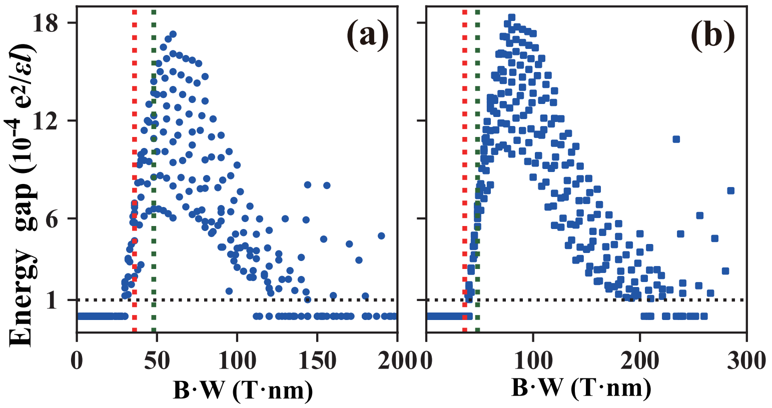


FIG. S4: The relation between $B \cdot W$ and the minimum gap. The data are from Fig. 2 in the main text. The red and green dot lines represents sample a and b in the expriment[1], respectively.

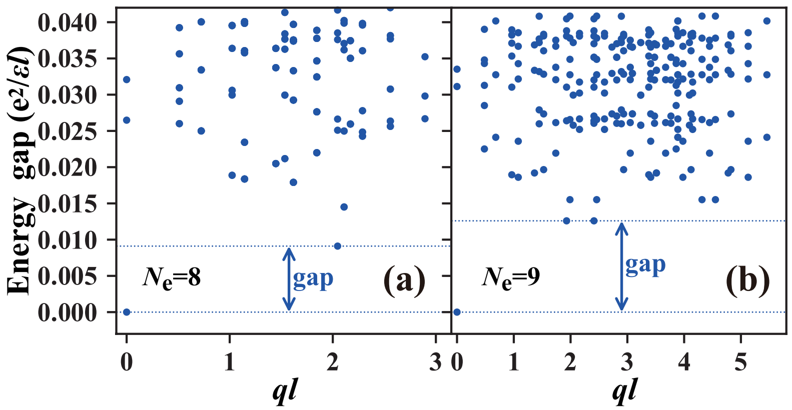


FIG. S5: The collective modes at $\nu = -4/3$, which corresponds to the valance band of black phosphorene. The magnetic field is $B = 45$ T. (a)$N_e = 8$ and (b) $N_e = 9$. The collective modes are not very much size-dependent. The 2DEG is incompressible with a minimum gap $\sim 1 \times 10^{-2} \frac{e^2}{\epsilon_{bp}\ell}$.

### E. Detailed data in black phosphorene

To be sure that the screening theory is correct, we exam the numerical data of $-4/3$ FQHE state in Fig. S5. The lowest collective mode is similar to that of the 2DEG in higher LLs in a conventional quantum well. It is incompressible, compatible with the experiment.

In Fig. S6, we indicate the collective modes of $\nu = \pm 5/2, \pm 7/2$ states in black phosphorene. As stated in the main text, none of them is stable.

In Fig. S7, we show the collective modes of $\nu = \pm 9/2$ and $\pm 11/2$ states in black phosphorene. The minimum gaps are as large as $10^{-3} \frac{e^2}{\epsilon \ell}$.

---

[1] Joseph Falson, Daniela Tabrea, Ding Zhang, Inti Sodemann, Yusuke Kozuka, Atsushi Tsukazaki, Masashi Kawasaki, Klaus von Klitzing, Jurgen H. Smet, Sci. Adv. **4**, eaat8742 (2018).

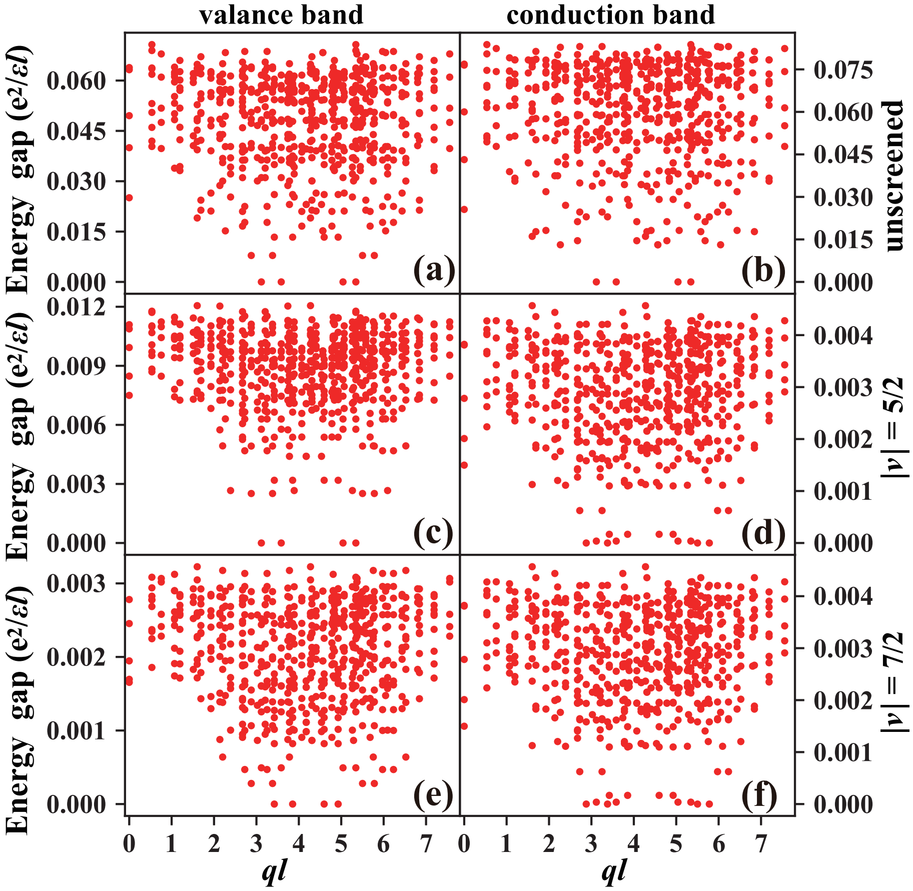


FIG. S6: The collective modes of $N_e = 11$ at (a) $\nu = -5/2$ and (b) $\nu = 5/2$ without screening at $B = 10$ T. These collective modes are also for $\nu = \pm 7/2$ since the screening is not considered. When the screening is added, the collective modes are changed: (c) $\nu = -5/2$ (d) $\nu = 5/2$, (e) $\nu = -7/2$, (f) $\nu = 7/2$.

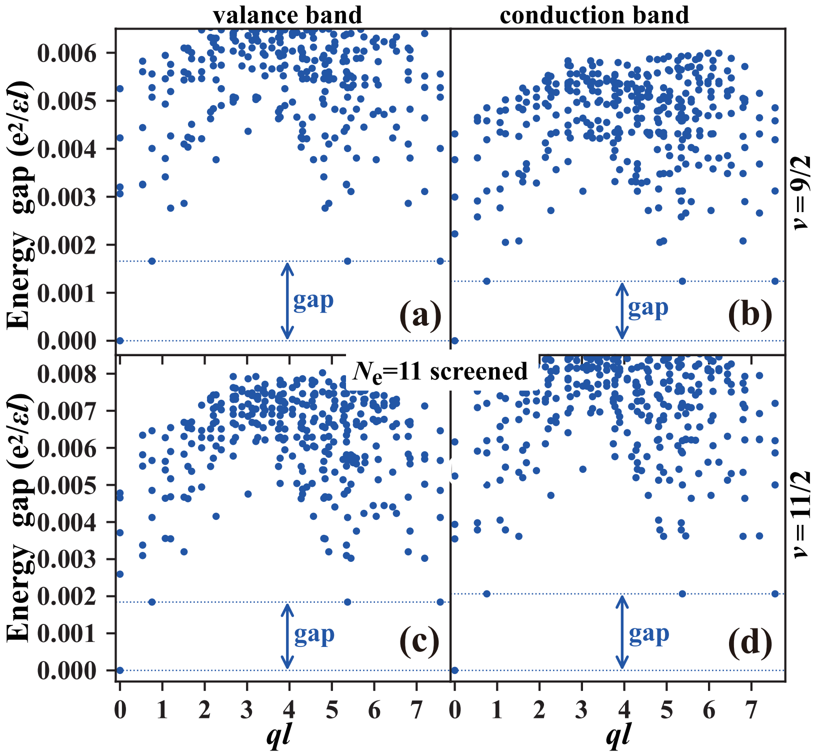


FIG. S7: The collective modes of $N_e = 11$ at (a) $\nu = -9/2$, (b) $\nu = 9/2$, (c) $\nu = -11/2$, and (d) $\nu = 11/2$ with screening at $B = 10$ T.
